# Supplementary material for: Evaluating Test-Time Scaling of General LLM Agents
Source: arXiv:2602.18998 source file (2026-09-29)
Supplement: Supplementary file 1 [file appendix_clarifactions.tex]

% \section{Clarifications}

% \begin{figure}[h]
%     \centering
%     \includegraphics[width=0.8\linewidth]{figs/model_pair_wise_consistency.pdf}
%     \caption{Models' spearman rank correlation across tasks}
%     \label{fig:model_pairwise_consistency}
% \end{figure}


% \subsection{Default context length and target context length}
% Default context length refers to the number of tokens in the final turn (including the input, conversation history, and the model’s final output) when the model is evaluated without any constraints.
% Target context length refers to a manually constrained context length (e.g., 8K, 16K, 32K, etc.) used to study the model’s performance under specific limitations.

% When the target context length is shorter than the default context length, we evaluate the model under a shorter context with fewer computational resources—this typically involves early-stopping the task.
% Conversely, when the target context length is longer than the default context length, we intentionally expand the model’s computation and encourage it to reason further. In this case, we prepend an “Expand” prompt before the model produces its final answer.

% \textbf{Expand prompt}: Before finalizing your answer, take additional time to verify your reasoning, consider alternative approaches, and search for any missing information that could strengthen your response.

% \textbf{Stop prompt}: **CRITICAL: You MUST provide your final answer immediately. Do NOT perform any more tool calling or reasoning. Return the final answer under the required format NOW.**

% \subsection{Eval configs}
% For the main experiments, evaluate according to the original dataset configurations; for the analysis, please standardize the parameters. 

% \begin{table}[h]
%     \centering
%     \begin{tabular}{lc}
%     \toprule
%         \textbf{Params} & \textbf{Value} \\
%     \midrule
%          Agent temperature & 0.7 \\
%          User agent temperature & 0.0 \\
%     \bottomrule
%     \end{tabular}
%     \vspace{2mm}
%     \caption{Parameters used for analysis}
% \end{table}

% *$\tau^2$-Bench need customer service agent and user agent for multi-round conversation.
