# Supplementary material for: Evaluating Test-Time Scaling of General LLM Agents
Source: arXiv:2602.18998 source file (2026-09-29)
Supplement: Supplementary file 2 [file appendix_cross_domain_tools.tex]

% \begin{tcolorbox}[
%   colback=gray!5,
%   colframe=gray!70,
%   title=\textbf{Case Study: Retrieving the Latest HuggingFace Model for Text Classification},
%   fonttitle=\bfseries\small,
%   fontupper=\ttfamily\scriptsize,
%   breakable
% ]

% \textbf{Task.}
% Identify the most recent pre-trained language model on HuggingFace suitable for text classification.

% \vspace{4pt}
% \hrule
% \vspace{6pt}

% \textbf{Plain Web Search Baseline (6 turns).}
% \begin{verbatim}
% Turn 1: <search> latest Hugging Face pre-trained language 
%         model text classification 2024 </search>
% Turn 2: <search> Hugging Face text classification models 
%         sorted by recent trending 2024 </search>
% Turn 3: <search> Hugging Face newest text classification 
%         models January 2025 recently released </search>
% ...
% Turn 6: <answer> tabularisai/multilingual-sentiment-analysis
%         (fine-tuned DistilBERT-base-multilingual-cased)
%         </answer>
% \end{verbatim}

% \vspace{4pt}
% \hrule
% \vspace{6pt}

% \textbf{General agent response with Specialized Tools (4 turns).}
% \begin{verbatim}
% Turn 1: Hugging_Face__search-models
%         {"tags": "text-classification", "limit": 15}
%         -> [{"id": "FutureMa/Qwen3-4B-Evasion", "downloads": 35},
%             {"id": "BAAI/bge-reranker-v2-m3", "downloads": 2807076}, ...]

% Turn 2: search__web_search "ModernBERT Hugging Face 2025"
%         -> "ModernBERT... 8,192-token context, 139M/395M params,
%            trained on 2T tokens"

% Turn 3: Hugging_Face__get-model-info
%         {"model_id": "answerdotai/ModernBERT-base"}
%         -> Full model card and architecture details
% \end{verbatim}

% \end{tcolorbox}
