# Supplementary material for: Evaluating Test-Time Scaling of General LLM Agents
Source: arXiv:2602.18998 source file (2026-09-29)
Supplement: Supplementary file 3 [file appendix_definition.tex]

## Appendix X: Theoretical Details for the Scaling Plateau

### A.1 Instance-Level Model

**Assumption 1** (Instance-level Bernoulli model). For each instance $b_i$ and context budget $c_k$, the $T$ independent evaluation outcomes $Y_{i,k}^{(1)}, \dots, Y_{i,k}^{(T)}$ are i.i.d. draws from $\text{Bernoulli}(p_{i,k})$.

**Assumption 2** (Independence across instances). Conditional on the model and context budget, outcomes across distinct instances are independent.

The population-level accuracy is $\mu_k = \frac{1}{N} \sum_{j=1}^{N} p_{j,k}$, estimated by $\hat{\mu}_k = \frac{1}{n} \sum_{i=1}^{n} \hat{p}_{i,k}$ where $\hat{p}_{i,k} = \frac{1}{T} \sum_{t=1}^{T} Y_{i,k}^{(t)}$.

### A.2 Variance Decomposition

The variance of $\bar{d}^{(k)}$ decomposes into two sources.

**Inference variance** (within-instance, due to stochastic decoding):

$$\text{Var}_{\text{inf}}(d_i^{(k)}) = \frac{p_{i,k+1}(1 - p_{i,k+1}) + p_{i,k}(1 - p_{i,k})}{T}$$

**Sampling variance** (across instances, due to subset selection):

$$\text{Var}_{\text{samp}}(\bar{d}^{(k)}) = \frac{\sigma_\delta^2}{n} \cdot \frac{N - n}{N - 1}$$

where $\sigma_\delta^2 = \frac{1}{N} \sum_{j=1}^{N} (\delta_j^{(k)} - \Delta_k)^2$ is the population variance of per-instance gains $\delta_j^{(k)} = p_{j,k+1} - p_{j,k}$.

The total variance combines both:

$$\text{Var}(\bar{d}^{(k)}) = \frac{1}{n} \left( \frac{\sigma_\delta^2 (N - n)}{N - 1} + \frac{1}{T} \cdot \frac{1}{N} \sum_{j=1}^{N} \left[ p_{j,k+1}(1 - p_{j,k+1}) + p_{j,k}(1 - p_{j,k}) \right] \right)$$

**Remark.** When $T = 1$, the inference and sampling components are not separately identifiable from observed data. The bootstrap over $\{d_1^{(k)}, \dots, d_n^{(k)}\}$ directly estimates the total variance, which is the correct target for CI construction.

### A.3 Finite Population Correction

The $n$ instances are drawn without replacement from $N$. The standard bootstrap resamples with replacement, targeting the with-replacement variance $\text{Var}_{\text{wr}} = S_d^2 / n$. The without-replacement variance satisfies:

$$\text{Var}_{\text{wor}} = \text{Var}_{\text{wr}} \cdot \frac{N - n}{N - 1}$$

Hence we multiply the bootstrap variance estimate by $\frac{N-n}{N-1}$.

### A.4 Asymptotic Validity

**Proposition 1** (Asymptotic normality). Under Assumptions 1–2, as $n \to \infty$ with $n/N \to \lambda \in (0,1)$:

$$\frac{\bar{d}^{(k)} - \Delta_k}{\sqrt{\text{Var}(\bar{d}^{(k)})}} \xrightarrow{d} \mathcal{N}(0, 1)$$

*Proof.* The paired differences $d_i^{(k)}$ are independent across instances (Assumption 2) and bounded in $[-1, 1]$, satisfying the Lindeberg condition. The result follows from the finite population CLT (Hájek, 1960).

**Proposition 2** (Bootstrap consistency). The corrected bootstrap variance estimator is consistent:

$$\hat{\sigma}^2_{\text{boot}} \cdot \frac{N-n}{N-1} \xrightarrow{p} \text{Var}(\bar{d}^{(k)})$$

*Proof.* The with-replacement bootstrap consistently estimates the variance of the sample mean for i.i.d. bounded random variables (Efron, 1979; Bickel & Freedman, 1981). Multiplying by the FPC $\frac{N-n}{N-1}$ yields a consistent estimator of the without-replacement variance.

**Corollary** (Coverage). Under the conditions above:

$$P\left( \Delta_k \in \text{CI}_k \right) \to 1 - \alpha$$

### A.5 Multiple Comparisons

Testing across $K-1$ consecutive pairs raises a multiple testing concern. However, since $k^*$ is defined as the *first* index where significance is lost, a fixed-sequence testing procedure applies: tests are conducted in order $k = 1, 2, \dots$, and we stop at the first non-rejection. This controls the family-wise error rate at level $\alpha$ without requiring Bonferroni or other corrections (Westfall & Krishen, 2001).

### A.6 Practical Recommendations

1. **Number of trials $T$.** $T = 1$ is valid but may yield wide CIs. If the scaling plateau cannot be clearly identified, increasing $T$ reduces inference noise and narrows CIs without requiring additional benchmark instances.

2. **Bootstrap iterations.** $B \geq 10{,}000$ is recommended for stable variance estimation.

3. **FPC magnitude.** For $n/N = 0.1$, the CI narrows by ${\sim}5\%$; for $n/N = 0.5$, by ${\sim}29\%$. The correction is non-negligible when $n/N > 0.05$.
