# Supplementary material for: Evaluating Test-Time Scaling of General LLM Agents
Source: arXiv:2602.18998 source file (2026-09-29)
Supplement: Supplementary file 4 [file appendix_details_domain_agents.tex]

\section{Details of the implementation.}

\subsection{Search Agent}

The search agent is currently a prompt only agent, meaning it doesn't utilize the API for tool calls. Tools are put into the prompt and parsed. It supports the following tools:
\begin{itemize}
\item \textbf{search}: search the web for information if you consider you lack some knowledge.
\item \textbf{answer}: output the final answer if you consider you are able to answer the question. The answer should be short and concise. No justification is needed.
\item \textbf{summary}: summarize the history turns. Reflect the search queries and search results in you history turns, and keep the information you consider important for answering the question and generating your report. Still keep the tag structure, $...$ The history turn information for your subsequent turns will be updated according to this summary action.
\item \textbf{think}: thinking process
\end{itemize}
There are two different prompts, one for internal thinking with no think tool, and one with external thinking with a think tool. zThe result of the search appends the search output within information tags which is fed back into the agent. 

\subsection{Coding Agent - OpenHands}

The coding agent OpenHands utilizes LiteLLM API as a unified API to call all language models. Tools are called through the API rather than in the prompt.
\begin{itemize}
\item \textbf{execute bash}: Execute a bash command in the terminal within a persistent shell session.
\item \textbf{str replace editor}: Custom editing tool for viewing, creating and editing files in plain-text format
\item \textbf{finish}: Signals the completion of the current task or conversation.
\item \textbf{task tracker}: This tool provides structured task management capabilities for development workflows.
It enables systematic tracking of work items, progress monitoring, and efficient
organization of complex development activities.
\item \textbf{think}: Use the tool to think about something. It will not obtain new information or make any changes to the repository, but just log the thought. Use it when complex reasoning or brainstorming is needed.
\end{itemize}

% \subsection{Math Agent - MathHay}


\subsection{Tool-calling Agent}
\subsubsection{$\tau^2$-Bench}
\paragraph{Framework} $\tau^2$-bench implements a simulation framework for evaluating customer service agents across various domains. This framework invloves \textbf{1) customer service agent}, the agent providing help with customer demands and \textbf{2) user agent}, giving responses to simulate human-like feedbacks in multi-round conversation. 

\paragraph{Evaluation} $\tau^2$-Bench uses binary evaluation (0/1) by comparing the agent's final environment state against a gold standard through environment replay. The reward is the product of multiple dimensions, covering database state, environment assertions, action sequences, and communication. A task succeeds only when all dimensions achieve 1.0, requiring exact database state matching via hash comparison and complete satisfaction of all assertions and action requirements. 

\paragraph{Datasets}
% types
% lite sampling
$\tau^2$-Bench provides 3 domains: airline, retail and telecom to simulate customer service conversation in real-life scenarios. Each domain contains a policy the agent must follow, a set of tools that agent can use and a set of tasks to evaluate the agent's performance. 

The original test set contains 50 tasks for airline domain, 114 tasks for retail and 114 tasks for telecom(midium version). Considering the cost of agents, We selected 10 tasks for airline domain, 20 tasks for retail domain and 20 tasks for telecom domain in our sampled test set accoridng to conversation length distribution. We first run the benchmark on gpt-oss-120B, Claude Sonnet 4.5 and Gemini-2.5-Pro models and get an estimation of conversation length for each task(measured by the length of last round input of customer service agent). Then we sample the data uniformly given the estimated length distribution to ensure the sampled dataset is representative in converastion length.


\paragraph{General Settings}
We choose gpt-oss-120B model as user agent simulator model. The temperature of user agent is set to 0.0 for stable human response simulation. The temperature of customer agent is set to 0.70 to encourage model to try different ways in solving problems. Please refer to Table~\ref{tab:tau2bench-hyperparams} for detailed hyperparameter settings. 
%$\tau^2$-Bench manage API calls using LiteLLM and we further add support for OpenAI platform and 

\begin{table}[]
\centering
% \scriptsize
\begin{tabular}{ll}
\toprule
\textbf{Parameter} & \textbf{Value} \\
\midrule
DEFAULT\_SEED & 300 \\
DEFAULT\_MAX\_STEPS & 2000 \\
DEFAULT\_MAX\_ERRORS & 10 \\
DEFAULT\_MAX\_CONCURRENCY & 3 \\
DEFAULT\_NUM\_TRIALS & 1 \\
DEFAULT\_AGENT\_IMPLEMENTATION & llm\_agent \\
DEFAULT\_USER\_IMPLEMENTATION & user\_simulator \\
DEFAULT\_LLM\_USER & gpt-oss-120B-1:0 \\
DEFAULT\_LLM\_TEMPERATURE\_AGENT & 0.70 \\
DEFAULT\_LLM\_TEMPERATURE\_USER & 0.00 \\
\bottomrule
\end{tabular}
\vspace{0.3cm}
\caption{$\tau^2$-Bench benchmark hyperparameters.}
\label{tab:tau2bench-hyperparams}
\end{table}


\paragraph{Parallel Scaling Settings}
% metric calculation bestk
% 为什么选8次
% metrics 看的是什么指标
For parallel scaling, we run the benchmark 8 times for each model and record past@$K$ results. We count results with rewards=1.0 as successful results. For each task, if the task is successfully solved at least once in first $k$ times running, past@$K$ of this task will be counted as 1. The final past@$K$ results are the average on all 50 tasks.


\paragraph{Sequential Scaling Settings}
% stop/extension strategy
% prompt
% budget selection
% metric calculation
In sequential scaling, we control the length of conversation by dynamically adding stop/extension prompts. 
% Please refer to Box~\ref{box:prompt-stop} and Box~\ref{box:prompt-extend} for detailed prompts. 
Since in $\tau^2$-Bench framework, the user agent controls the ending of the conversation by sending end-signals, we implement the dynamic strategy in user agent simulator. Our strategy dynamically injects stop or extension prompts based on both agent intent and token usage. It consists of two parts: \textbf{1) Add STOP prompt.} The simulator monitors cumulative context tokens against a configurable budget and intercepts user messages to detect explicit end-signals(signal of transferring to human operator, conversation out of scope or simply stop). If the budget is reached, it emits a soft stop by appending a directive STOP\_PROMPT and defers the actual end-signal to the next turn via a ready-stop flag. Notice that the stopping strategy will allow the customer service agent act for another round and force user simulator to terminate the conversation by sending end-signal in the next turn. \textbf{2) Add EXTEND prompt.} If the user attempts to stop before the budget is exhausted, we will cleans the end-signal and  appends an EXTEND\_PROMPT that nudges the agent to deepen reasoning, verify outputs, and seek missing evidence. 

\begin{tcolorbox}[
  colback=gray!5,
  colframe=gray!70,
  title=\textbf{Stop Prompt},
  fonttitle=\bfseries\small,
  breakable
]
**CRITICAL: You MUST provide your final answer immediately. Do NOT perform any more tool calling or reasoning. Return the final answer under the required format NOW.**
\end{tcolorbox}

\begin{tcolorbox}[
  colback=gray!5,
  colframe=gray!70,
  title=\textbf{Extension Prompt},
  fonttitle=\bfseries\small,
  breakable
]
Before finalizing your answer, take additional time to verify your reasoning, consider alternative approaches, and search for any missing information that could strengthen your response.
\end{tcolorbox}



\subsubsection{MCP-Bench}
\paragraph{Framework.}
For each benchmark instance, MCP-Bench presents the agent with a fuzzy natural language task description and a large MCP tool ecosystem consisting of relevant servers plus distractor servers. The agent then interacts with this environment in a multi-round plan–execute loop: at each step it selects one or more tools, constructs structured arguments that respect the MCP schema, and invokes these tools to obtain intermediate results. The raw tool outputs are optionally compressed into shorter summaries to control context length while preserving information needed for downstream decisions. These summaries, together with the original outputs and previous actions, are appended to an execution trace that forms the agent’s internal state. The agent iteratively updates this state, revises its plan, and decides whether to continue calling tools or terminate. Once it judges the task to be complete, it produces a final natural language answer conditioned on the accumulated execution trace.

\paragraph{Evaluation.}
The evaluation pipeline combines rule-based execution checks with rubric-based LLM-as-a-Judge scoring, and summarizes performance along four axis-level scores. Rule-based metrics are computed directly from the tool-call trace, covering valid tool naming, input-schema adherence, runtime success, and dependency compliance. The LLM judge is then prompted with the fuzzy task description, the hidden concrete task specification and dependency analysis, the summarized execution trajectory, and the final answer, and assigns rubric-based scores along higher-level dimensions. There are four axis scores:
\textbf{1) Schema Understanding Score} includes Valid Tool Name Rate ($s_{\text{name}})$, Schema Compliance ($s_{\text{schema}}$) and Execution Success ($ s_{\text{execution}}$). Captures the agent’s low-level robustness in handling tool interfaces, aggregating valid tool name rate, schema compliance rate, and execution success rate into a single score that reflects how reliably the agent issues well-formed, executable calls.
\textbf{2) Task Completion Score} includes Task Fulfillment ($s_{\text{fulfillment}}$) and Information Grounding ($s_{\text{grounding}}$). Measures whether the agent actually solves the task, based on LLM-judge sub-dimensions such as task fulfillment, coverage of required subtasks, information grounding in tool outputs, and overall answer relevance.
\textbf{3) Tool Usage Score} includes Tool Appropriateness ($s_{\text{appropriateness}}$) and Parameter Accuracy ($s_{\text{parameter}}$). Evaluates how appropriately the agent selects and parameterizes tools, combining rubric scores for tool appropriateness (matching tools to subtasks) and parameter accuracy (correct and sufficient arguments for each call).
\textbf{4) Planning Effectiveness Score} includes Dependency Awareness($s_{\text{dependency}}$) and Parallelism and Efficiency($s_{\text{efficiency}}$). Assesses the structural quality of multi-round execution, including dependency awareness: respecting inter-tool ordering and data flow; and parallelism and efficiency: avoiding redundant calls and exploiting safe concurrency when possible. Considering sequential scaling settings, we excluded parallelism and efficiency score and only take dependency awareness into account.

Each score is normalized to $[0,1]$ and the final benchmark score for a model on a given setting is given as:

\begin{equation}
    S_{\text{overall}}
    = \frac{1}{2} \left(
        \frac{
        s_{\text{name}}+
        s_{\text{schema}}+
        s_{\text{execution}}
        }{3} + 
        \frac{
        s_{\text{fulfillment}}+
        s_{\text{grounding}}+
        s_{\text{appropriateness}}+
        s_{\text{parameter}}+
        s_{\text{dependency}}+
        s_{\text{efficiency}}
        }{5}
      \right).
\end{equation}

\paragraph{Datasets}
MCP-Bench requires the agent to solve the problem using 1 or 2 or 3 server, thus dividing the dataset into 3 subsets accordingly. Considering the tradeoff between data variaty and cost, we select 1 problem per server combination, which totals 52 tasks with 28 1-server tasks, 15 2-server tasks and 9 3-server tasks. 

\begin{table}[t]
\centering
% \scriptsize
\begin{tabular}{lll}
\toprule
\textbf{Category} & \textbf{Key} & \textbf{Value} \\
\midrule
\multirow{11}{*}{execution} & task\_timeout & 5000 \\
& task\_retry\_max & 1 \\
& retry\_delay & 5 \\
& compression\_retries & 1 \\
& max\_execution\_rounds & 2000 \\
& server\_semaphore\_limit & 20 \\
& context\_budget & null \\
& content\_summary\_threshold & 1000 \\
& content\_truncate\_length & 4000 \\
& error\_truncate\_length & 1000 \\
& error\_display\_prefix & 200 \\
\midrule
\multirow{3}{*}{evaluation} & judge\_stability\_runs & 5 \\
& judge\_model.name & gpt-oss-120B \\
& judge\_model.provider & LiteLLM \\
\midrule
\multirow{9}{*}{llm} & temperature & 0.7 \\
& json\_retry\_groups & 5 \\
& token\_reduction\_factors & [0.9, 0.8, 0.7] \\
& min\_tokens & 1000 \\
& token\_increment & 1000 \\
& format\_conversion\_tokens & 8000 \\
& planning\_tokens & 12000 \\
& summarization\_max\_tokens & 10000 \\
& user\_prompt\_max\_length & 30000 \\
\bottomrule
\end{tabular}
\vspace{0.2cm}
\caption{MCP-Bench configuration summary.}\label{tab:mcpbench_config}
\end{table}

\paragraph{General Settings} 
Table~\ref{tab:mcpbench_config} shows general settings for MCP-Bench. In case sequential scaling is early stopped by max\_execution\_rounds, we set its upper bounds well beyond the conversation rounds in sequential scaling. And we choose gpt-oss-120B as evaluator (different from o4-mini, gpt-4o and gpt-4o-mini) and run 5 times for each task to get a stable evaluation. Please refer to Table~\ref{app:tab:mcpbench-config} for detailed settings.

\begin{table*}[]
\centering
% \scriptsize
\begin{tabular}{lll}
\toprule
Category & Key & Value \\
\midrule
\multirow{6}{*}{mcp.connection} & http\_timeout & 60 \\
& tool\_discovery\_timeout & 10 \\
& server\_startup\_timeout & 30 \\
& health\_check\_timeout & 2 \\
& process\_wait\_timeout & 5 \\
& batch\_timeout & 60 \\
\midrule
\multirow{11}{*}{execution} & task\_timeout & 5000 \\
& task\_retry\_max & 1 \\
& retry\_delay & 5 \\
& compression\_retries & 1 \\
& max\_execution\_rounds & 2000 \\
& server\_semaphore\_limit & 20 \\
& context\_budget & null \\
& content\_summary\_threshold & 1000 \\
& content\_truncate\_length & 4000 \\
& error\_truncate\_length & 1000 \\
& error\_display\_prefix & 200 \\
\midrule
\multirow{3}{*}{evaluation} & judge\_stability\_runs & 5 \\
& judge\_model.name & gpt-oss-120B \\
& judge\_model.provider & LiteLLM \\
\midrule
\multirow{9}{*}{llm} & temperature & 0.7 \\
& json\_retry\_groups & 5 \\
& token\_reduction\_factors & [0.9, 0.8, 0.7] \\
& min\_tokens & 1000 \\
& token\_increment & 1000 \\
& format\_conversion\_tokens & 8000 \\
& planning\_tokens & 12000 \\
& summarization\_max\_tokens & 10000 \\
& user\_prompt\_max\_length & 30000 \\
\midrule
\multirow{10}{*}{data\_collection} & individual\_timeout & 30 \\
& batch\_timeout & 60 \\
& max\_retries & 2 \\
& retry\_delay\_base & 3 \\
& retry\_delay\_multiplier & 2 \\
& batch\_retry\_delay\_base & 5 \\
& batch\_retry\_delay\_multiplier & 3 \\
& default\_http\_port & 3000 \\
& tool\_description\_truncate & 150 \\
& (no\_cache\_fields\_here) & - \\
\midrule
\multirow{2}{*}{task\_generation} & tasks\_per\_combination & 1 \\
& generation\_max\_retries & 1 \\
\midrule
\multirow{2}{*}{dependency\_extraction} & required\_support\_count & 3 \\
& min\_support\_count & 2 \\
\midrule
\multirow{2}{*}{server\_selection} & selection\_tokens & 8000 \\
& tool\_sample\_count & 3 \\
\bottomrule
\end{tabular}
\caption{MCP-Bench configuration summary.}\label{app:tab:mcpbench-config}
\end{table*}


\paragraph{Parallel Scaling Settings}
Similar to $\tau^2$-Bench, we run MCP-Bench for 4 times on each model and record past@$K$ results. For each task, we choose the highest $S_{\text{overall}}$ in first $k$ runs as the past@$K$ score for this task. Then we average past@$K$ scores from 52 tasks as final past@$k$ score. 


\paragraph{Sequential Scaling Settings} 
In sequential scaling, we control conversation length by dynamically adding stop/extension prompts during multi-round execution. Stop prompt and extension prompt are the same as $\tau^2$-Bench. 
% Please refer to Box~\ref{box:prompt-stop} and Box~\ref{box:prompt-extend} for detailed prompts. 

In MCP-Bench, the decision loop is implemented inside the executor. Our strategy injects STOP or EXTEND prompts based on agent intent and token usage tracked per round. It consists of two parts: \textbf{1) Add STOP prompt.} Before each planning call, the executor estimates this round’s prompt tokens against a configurable context\_budget. If the estimated prompt for the current round would exceed the budget, it appends a STOP\_PROMPT to the planning prompt, sets force\_stop, and prevents new tool executions (planned\_tools cleared). When the agent signals stop without a budget, the executor terminates the loop. \textbf{2) Add EXTEND prompt.} If the agent attempts to stop while the budget still permits another round, the executor estimates the next round’s cost as current\_round\_tokens plus the EXTEND\_PROMPT tokens. If within budget, it sets an extend\_next\_round flag, flips should\_continue to true for this turn, and injects EXTEND\_PROMPT into the next round’s planning prompt, nudging the agent to deepen reasoning, verify outputs, and seek missing evidence. 

For token budget choices, we first use gpt-oss-120B to estimate context length of the task (measured by the context length of the last round conversation input) and we find the context length varies across 1-server, 2-server and 3server tasks. Generally, for 1-server tasks, the context length is shorter than that of 3-server due to task complexity. If we select fixed length for all 3 servers, some choices of small token budgets will stop the conversation in complex tasks even before the first round conversation ends; some larger budgets will still extend the conversation even though the problem has been solved with shorter context. Therefore, we select different scale in sequential scaling: 8k-32k for 1-server, 16k-64k for 2-server and 24k-96k for 3-server.

% \subsection{MCP Agent}
% \subsubsection{$\tau^2$-Bench}
% $\tau^2$-bench is a dual-control simulation framework for evaluating customer service agents in 3 scenarios: airline, retail and telecom. There are two roles in this system: an user for human-like response and an agent for customer service. The simulation environment is from databases based on local json files, such as user info and flight info. The bench also designed several tools for each specific domains locally. The evaluation is both rule-based and LLM-as-Judge. $\tau$-Bench use LiteLLM to manage API calls. 


% \begin{table}[h!]
% \centering
% \small
% \begin{tabular}{llp{6cm}c}
% \toprule
% \textbf{Domain} & \textbf{Tool Type} & \textbf{APIs} & \textbf{Total} \\
% \midrule

% \multirow{3}{*}{\textbf{Airline}} 
% & Agent Tools & Book Reservation, Calculate, Cancel Reservation,...
% %Get Reservation Details, Get User Details, List All Airports, Search Direct Flight, Search Onestop Flight, Send Certificate, Transfer To Human Agents, Update Reservation Baggages, Update Reservation Flights, Update Reservation Passengers, Get Flight Status 
% & 14 \\
% & User Tools  & --- & 0 \\

% \midrule

% \multirow{3}{*}{\textbf{Retail}} 
% & Agent Tools & Calculate, Cancel Pending Order, Exchange Delivered Order Items, ...
% %Find User Id By Name Zip, Find User Id By Email, Get Order Details, Get Product Details, Get User Details, List All Product Types, Modify Pending Order Address, Modify Pending Order Items, Modify Pending Order Payment, Modify User Address, Return Delivered Order Items, Transfer To Human Agents 
% & 15 \\
% & User Tools  & --- & 0 \\

% \midrule

% \multirow{5}{*}{\textbf{Telecom}} 
% & Agent Tools & Get Customer By Phone, Get Customer By Id, Get Customer By Name, Get Details By Id, 
% %Suspend Line, Resume Line, Get Bills For Customer, Send Payment Request, Get Data Usage, Enable Roaming, Disable Roaming, Transfer To Human Agents, Refuel Data 
% & 13 \\
% & User Tools & Check Status Bar, Check Network Status, Check Network Mode Preference, 
% %Set Network Mode Preference, Run Speed Test, Toggle Airplane Mode, Check Sim Status, Reseat Sim Card, Toggle Data, Toggle Roaming, Check Data Restriction Status, Toggle Data Saver Mode, Check Apn Settings, Set Apn Settings, Reset Apn Settings, Check Wifi Status, Toggle Wifi, Check Wifi Calling Status, Toggle Wifi Calling, Check Vpn Status, Connect Vpn, Disconnect Vpn, Check Installed Apps, Check App Status, Check App Permissions, Grant App Permission, Can Send Mms, Reboot Device, Check Payment Request, Make Payment 
% & 30 \\

% \bottomrule
% \end{tabular}
% \vspace{0.5em}
% \caption{Overview of Available Tools across Domains in $\tau^2$-Bench}

% \end{table}


% \subsubsection{MCP-Bench}
% MCP generally follows: 1. LLMs send request 2. MCP server receives request and processes request 3. Return execution results to LLMs with standard format.For MCP-Bench, there are 28 MCP servers and 246 tools in total. Table \ref{tab:mcp-bench-tools} lists server name and their tools. Evaluations are based on LLM-as-Judge. LiteLLM was added to manage API calls.

% %But the \hyperlink{https://clinicaltrialsapi.cancer.gov/signin}{login system on National Cancer Institute(NIH)} website  seems to be broken(?).

% \begin{table}[h]
% \centering
% \small
% \begin{tabular}{lp{7cm}r}
% \toprule
% \textbf{Server} & \textbf{Tools (partial)} & \textbf{Total} \\
% \midrule

% BioMCP & search, fetch, think, article\_searcher, % trial\_searcher, trial\_getter, trial\_protocol\_getter, trial\_references\_getter, trial\_outcomes\_getter, trial\_locations\_getter, variant\_searcher, variant\_getter, alphagenome\_predictor, gene\_getter, disease\_getter, drug\_getter, nci\_organization\_searcher, nci\_organization\_getter, nci\_intervention\_searcher, nci\_intervention\_getter, nci\_biomarker\_searcher, nci\_disease\_searcher, openfda\_adverse\_searcher, openfda\_adverse\_getter, openfda\_label\_searcher, openfda\_label\_getter, openfda\_device\_searcher, openfda\_device\_getter, openfda\_approval\_searcher, openfda\_approval\_getter, openfda\_recall\_searcher, openfda\_recall\_getter, openfda\_shortage\_searcher, openfda\_shortage\_getter
% & 35 \\

% Scientific Computing & create\_tensor, view\_tensor, delete\_tensor, add\_matrices, % subtract\_matrices, multiply\_matrices, scale\_matrix, matrix\_inverse, transpose, determinant, rank, compute\_eigen, qr\_decompose, svd\_decompose, find\_orthonormal\_basis, change\_basis, vector\_project, vector\_dot\_product, vector\_cross\_product, gradient, curl, divergence, laplacian, directional\_deriv, plot\_vector\_field, plot\_function
% & 26 \\

% Medical Calculator & egfr\_epi, egfr\_epi\_cr\_cys, bp\_children, bmi\_bsa\_calculator, % crcl\_cockcroft\_gault, map\_calculator, chads2\_vasc\_score, prevent\_cvd\_risk, corrected\_calcium, qtc\_calculator, wells\_pe\_criteria, ibw\_abw\_calculator, pregnancy\_calculator, revised\_cardiac\_risk\_index, child\_pugh\_score, steroid\_conversion, calculate\_mme, maintenance\_fluids, corrected\_sodium, meld\_3, framingham\_risk\_score, homa\_ir
% & 22 \\

% NASA Data & get\_astronomy\_picture\_of\_day, get\_asteroids\_feed, get\_asteroid\_lookup, browse\_asteroids, % get\_coronal\_mass\_ejection, get\_geomagnetic\_storm, get\_solar\_flare, get\_solar\_energetic\_particle, get\_magnetopause\_crossing, get\_radiation\_belt\_enhancement, get\_hight\_speed\_stream, get\_wsa\_enlil\_simulation, get\_notifications, get\_earth\_imagery, get\_earth\_assets, get\_epic\_imagery, get\_epic\_imagery\_by\_date, get\_epic\_dates, get\_exoplanet\_data, get\_mars\_rover\_photos, get\_mars\_rover\_manifest
% & 21 \\

% Paper Search & search\_arxiv, search\_pubmed, search\_biorxiv, search\_medrxiv, % search\_google\_scholar, search\_iacr, download\_arxiv, download\_pubmed, download\_biorxiv, download\_medrxiv, download\_iacr, read\_arxiv\_paper, read\_pubmed\_paper, read\_biorxiv\_paper, read\_medrxiv\_paper, read\_iacr\_paper, search\_semantic, download\_semantic, read\_semantic\_paper
% & 19 \\

% NixOS & nixos\_search, nixos\_info, nixos\_channels, nixos\_stats, % home\_manager\_search, home\_manager\_info, home\_manager\_stats, home\_manager\_list\_options, home\_manager\_options\_by\_prefix, darwin\_search, darwin\_info, darwin\_stats, darwin\_list\_options, darwin\_options\_by\_prefix, nixos\_flakes\_stats, nixos\_flakes\_search, nixhub\_package\_versions, nixhub\_find\_version
% & 18 \\

% Unit Converter & convert\_temperature, convert\_angle, convert\_length, convert\_energy, % convert\_force, convert\_pressure, convert\_power, convert\_speed, convert\_area, convert\_mass, convert\_volume, convert\_computer\_data, convert\_density, convert\_time, convert\_batch, list\_supported\_units
% & 16 \\

% Math MCP & add, subtract, multiply, division, % sum, mean, median, mode, min, max, floor, ceiling, round
% & 13 \\

% DEX Paprika & getNetworks, getNetworkDexes, getNetworkPools, getDexPools, % getPoolDetails, getTokenDetails, getTokenPools, getPoolOHLCV, getPoolTransactions, search, getStats
% & 11 \\

% Hugging Face & search-models, get-model-info, search-datasets, get-dataset-info, % search-spaces, get-space-info, get-paper-info, get-daily-papers, search-collections, get-collection-info
% & 10 \\

% Google Maps & search\_nearby, get\_place\_details, maps\_geocode, maps\_reverse\_geocode, % maps\_distance\_matrix, maps\_directions, maps\_elevation
% & 7 \\

% Game Trends & get\_steam\_trending\_games, get\_steam\_top\_sellers, get\_steam\_most\_played, get\_epic\_free\_games, % get\_epic\_trending\_games, get\_all\_trending\_games, get\_api\_health
% & 7 \\

% OSINT Intelligence & whois\_lookup, nmap\_scan, dnsrecon\_lookup, dnstwist\_lookup, % dig\_lookup, host\_lookup, osint\_overview
% & 7 \\

% National Parks & findParks, getParkDetails, getAlerts, getVisitorCenters, % getCampgrounds, getEvents
% & 6 \\

% Bibliomantic & i\_ching\_divination, bibliomantic\_consultation, get\_hexagram\_details, server\_statistics
% & 4 \\

% Weather Data & get\_current\_weather\_tool, get\_weather\_forecast\_tool, search\_locations\_tool, get\_live\_temp
% & 4 \\

% Car Price Evaluator & get\_car\_brands, search\_car\_price, get\_vehicles\_by\_type
% & 3 \\

% Huge Icons & list\_icons, search\_icons, get\_platform\_usage
% & 3 \\

% Metropolitan Museum & list-departments, search-museum-objects, get-museum-object
% & 3 \\

% OpenAPI Explorer & getApiOverview, getApiOperation
% & 2 \\

% Context7 & resolve-library-id, get-library-docs
% & 2 \\

% OKX Exchange & get\_price, get\_candlesticks
% & 2 \\

% Time MCP & get\_current\_time, convert\_time
% & 2 \\

% Call for Papers & get\_events
% & 1 \\

% FruityVice & get\_fruit\_nutrition
% & 1 \\

% Movie Recommender & get\_movies
% & 1 \\

% Wikipedia & --- & 0 \\

% Reddit & --- & 0 \\

% \bottomrule
% \end{tabular}
% \label{tab:mcp-bench-tools}
% \caption{Summary of MCP Servers and Tool Counts}
% \end{table}
% \clearpage




% \subsection{Unified Agent}

% The unified agent unifies all the agents together under a single framework, meaning a single agent with access to tool calls for all the different tasks. We will try to combine the system prompts of all the different agents together into a single system prompt that will work for all tasks. We expect performance to decrease, but maybe we can derive insights from this practice.\\
% \andy{
% Implementation will be quite tough, as the different agents call tools in different ways, TBD how to approach this.
% }

% \section{Analysis}

% \subsection{Test-Time Scaling}

% For test-time scaling, we will analyze:
% \begin{itemize}
% \item \textbf{Context Length:} This is the total length of a trajectory of an agent, including the following components:
% \begin{itemize}
% \item System prompt
% \item Question Input
% \item Model Output and Tool-Calls over multiple iterations (not including reasoning)
% \item Environment Output
% \end{itemize}
% \item \textbf{Avg. Reasoning Tokens per Iteration}: This is the average amount of reasoning tokens for each iteration of agent:
% \begin{itemize}
% \item For close-sourced models, reasoning tokens is outputted by the API or LiteLLM
% \item For open-source models (besides R1), there is no notion of reasoning. We will use think tags to simulate reasoning within the output. These reasoning tokens will not be fed in to later iterations of the agent, to stay in line with closed-source models. However, this is a departure from the REACT agent framework.
% \end{itemize}
% \end{itemize}
% \andy{
% Search agent might need to be edited to not feed back in the reasoning for open-source models
% }

% \subsection{Lexical Analysis}

% Current work by Pranav keeps track of "reasoning words" within different categories:
% \begin{itemize}
% \item \textbf{Planning/Directive}: "let me", "i should", "i need to", "the goal is", "first", "next", "then", "the plan is", "now i will"
% \item \textbf{Hesitation/Correction}: "wait", "maybe", "alternatively", "hmm", "perhaps"
% \item \textbf{Cognitive/Assertive}: "i think", "it seems", "this means", "therefore", "however", "based on", "okay", "good"
% \end{itemize}
% Then we plot the following for each model:
% \begin{itemize}
% \item avg. reasoning words per trajectory
% \item avg. count of each category of reasoning words per trajectory
% \item avg. reasoning words vs. accuracy
% \end{itemize}
% \andy{
% This metric doesn't seem like it'll work for the closed-source models, since we don't have access to the reasoning trace?
% }
% \xiaochuan{Yes. We can only do this analysis on open-source models.}

% \subsection{Reflection Ability (to be finalized)}

% We observe that models in agentic tasks tend to spend substantial time planning initially and rarely revise their plans later—showing limited reflection or self-correction. The models often appear highly confident in their initial answers.

% This may relate to entropy analysis: early tokens exhibit higher entropy (representing planning), while later tokens show lower entropy (execution).
% A possible experiment is to manually add an instruction such as “Double-check your answer and adjust your plan,” then measure the proportion of cases where the model changes its response:
% \begin{itemize}
%     \item From wrong → correct
%     \item From correct → wrong
%     \item From wrong → wrong (ineffective reflection)
% \end{itemize}

% \subsection{Sparse Attention}
