# Supplementary material for: Evaluating Test-Time Scaling of General LLM Agents
Source: arXiv:2602.18998 source file (2026-09-29)
Supplement: Supplementary file 5 [file appendix_domain_detailed_analysis.tex]

% \subsection{Per trajectory analysis}

% To understand the mechanisms driving the performance drop observed in sequential scaling, we conduct a granular analysis of agent trajectories. We utilize the $\tau^2$-Bench tool-use domain as a case study, plotting per-example accuracy across the sequential scaling dimension.As illustrated in Figure~\ref{fig:tau2-heatmap}, the heatmap of per-task outcomes (blue=success, red=failure) reveals a prevalent false $\to$ true $\to$ false pattern. While performance initially improves with additional computation, further scaling frequently leads to regression. Specifically, in $\tau^2$-Bench, 17 tasks that succeed at a 12K token budget fail at 22K (whereas only 14 tasks show improvement). Our analysis identifies three distinct failure modes responsible for this destabilization:

% \textbf{Preference Drift}: Increased reasoning space often leads agents to lose track of initial user constraints. For instance, in an airline retail task, a user specifies a preference for "RGB backlight, otherwise non-backlit." At a 12K budget, the agent correctly identifies the absence of RGB and selects a non-backlit item. However, at 22K, the agent inexplicably selects a white-backlit variant—a choice explicitly excluded by the user—despite having access to the same tool outputs.

% \textbf{Input Over-correction}: Larger contexts appear to encourage agents to "hallucinate" helpfulness by modifying verbatim user inputs. In one instance, a user provides the name "Mei Kovacs." While the 12K agent processes the name correctly, the 22K agent "corrects" the input to "Kovács" by adding Hungarian diacritics. This modification causes the subsequent database lookup to fail, resulting in a "User not found" error.

% \textbf{Action Loops}: Excessive computational budget can facilitate repetitive, unproductive behaviors. In a mobile troubleshooting scenario, a 12K agent calls transfer\_to\_human\_agents once before successfully resolving the issue within 29 total calls. In contrast, the 22K agent enters a pathological loop, executing 96 consecutive calls to the transfer tool, effectively exhausting the budget without reaching a resolution.


\subsection{Tool-calling}
\subsubsection{Parallel Scaling}
Figure~\ref{fig:parallel} shows the past@$K$ score changes with the increase of Round K. In both benchmarks, parallel rounds consistently improve past@$K$: moving from $K=1$ to $K=2$ and $K=4$ yields the largest gains, while the step from $K=4$ to $K=8$ gives only modest additional improvement, indicating diminishing returns from more parallel tool-call batches. On MCP-Bench, the models form a tight band, with gpt-oss-120B and Gemini-2.5-Flash slightly ahead across all $K$, Qwen3-235B and Qwen3-Next close behind, and DeepSeek-V3.2 consistently the weakest but still improving with larger $K$. On $\tau^2$-bench, the ranking spreads out more clearly: gpt-oss-120B dominates at every $K$, Gemini-2.5-Flash and Qwen3-235B occupy a strong middle cluster, DeepSeek-V3.2 is slightly below but broadly competitive, whereas Qwen3-Next lags substantially even at $K=8$. Comparing sparse-attention models to full-attention models, both Qwen3-Next and DeepSeek-V3.2 benefit from increased parallel rounds, but DeepSeek-V3.2 largely mirrors the scaling pattern of the stronger full-attention models, while Qwen3-Next shows much weaker scaling on $\tau^2$-bench and only partially closes the gap on MCP-Bench. Refer to Appendix~\ref{app:results-parallel-sequential} for detailed experiment results.


\begin{figure}[t]
\centering
\includegraphics[width=0.4\linewidth]{figs/tau2_parallel.png}
\includegraphics[width=0.4\linewidth]{figs/mcp_parallel.png}
\caption{$\tau^2$-Bench and MCP-Bench parallel scaling results.}
\label{fig:parallel}
\end{figure}



\subsubsection{Sequential Scaling}
On $\tau^2$-bench, sequential scaling typically shows a rise–then–fall pattern as the token budget increases: for example, with 2 servers, gpt-oss-120B and Gemini-2.5-Flash both improve steadily from the lowest budget up to the mid range (e.g., around 32–48K tokens), but their accuracy then plateaus or slightly decreases at the largest budget, and a similar peak-and-drop trend appears for Qwen3-235B and DeepSeek-V3.2. MCP-Bench exhibits the same qualitative behavior when multiple servers are used: with 2 servers, all models improve from 16K to 32–48K tokens and then show reduced accuracy at 64K, while with 3 servers, accuracy peaks around 48K and subsequently declines at 64K and 96K for every model, including the strongest one (Gemini-2.5-Flash) and weaker ones such as Qwen3-Next and DeepSeek-V3.2. For models trained using sparse attention, Qwen3-Next and DeepSeek-V3.2 trace out essentially the same rise–then–fall curves as the full-attention baselines across server counts and token budgets, but they tend to occupy the lower part of the accuracy range, particularly beyond the mid-range budgets where performance starts to drop.

\begin{figure}[t]
\centering
\includegraphics[width=0.4\linewidth]{figs/tau2_sequential.png}
\caption{$\tau^2$-Bench sequential scaling results.}
\label{fig:tau2bench-sequential}
\end{figure}

\begin{figure*}[t]
\centering
\includegraphics[width=0.9\linewidth]{figs/mcp_sequential.png}
\caption{MCP-Bench sequential scaling results.}
\label{fig:mcpbench-sequential}
\end{figure*}

\subsection{MCP-Bench efficiency axes degrade under higher budgets}
In MCP-Bench (3-server), increasing the budget from 48k to 96k does not translate into higher per-task overall quality for validly loaded tasks; instead, performance declines are concentrated on efficiency-oriented axes. Axis-level breakdown shows the two most affected dimensions are \textbf{Tool Usage} and \textbf{Planning}: Tool Usage exhibits the largest drop (e.g., $-0.124$), and Planning also decreases substantially (e.g., $-0.087$), while Schema stays nearly unchanged and Task only mildly declines. Execution traces suggest the degradation is driven by \textbf{over-exploration} that manifests as a \textbf{tool-call explosion} (mean tool-call ratio $\approx 5.34\times$ at 96k vs 48k), including duplicated searches, redundant retries, and the repeated use of placeholder/invalid intermediate IDs. As a result, the agent often spends additional steps on verification-like activity without improving decision quality, producing characteristic false $\rightarrow$ true $\rightarrow$ false trajectories as the budget increases—mid-range improvements can occur when exploration happens to align, but the dominant effect at higher budgets is reduced efficiency captured primarily by Tool Usage and Planning.

\begin{figure*}[t]
\centering
\includegraphics[width=0.4\linewidth]{figs/mcpbench_heatmap.png}
\caption{MCP-Bench overall score heatmap of sequential scaling.}
\label{fig:mcpbench-sequential}
\end{figure*}

\subsection{Case study}

We observe that models in agentic tasks tend to spend substantial time planning initially and rarely revise their plans later—showing limited reflection or self-correction. The models often appear highly confident in their initial answers.

This may relate to entropy analysis: early tokens exhibit higher entropy (representing planning), while later tokens show lower entropy (execution).
A possible experiment is to manually add an instruction such as “Double-check your answer and adjust your plan,” then measure the proportion of cases where the model changes its response:
\begin{itemize}
    \item From wrong → correct
    \item From correct → wrong
    \item From wrong → wrong (ineffective reflection)
\end{itemize}

Another observation could be models that remain confident and refuse to spend additional tokens on double-checking.


\subsubsection{Tool-calling}
%==============================================================================
\paragraph{Case A: Preference Drift}
\begin{itemize}
    \item \textbf{Setting:} $\tau^2$-Bench, Retail Domain, Task 0, Gemini-2.5-Flash. User requests a keyboard exchange with specific backlight preferences.
\end{itemize}
Refer to Box~\ref{box:caseA-12k} and Box~\ref{box:caseA-22k}.



\begin{tcolorbox}[
  colback=gray!5,
  colframe=gray!70,
  title=\textbf{12K Budget (Success)},
  fonttitle=\bfseries\small,
  breakable
]
\textbf{[User]:} I'd like to swap the keyboard I received for a similar full-size model with clicky switches. If there's a version that also has \textbf{RGB backlighting}, that would be ideal; otherwise I'm fine with a \textbf{non-backlit} clicky keyboard. \\[0.5em]
... \\[0.5em]
\textbf{[Assistant]:} I found the following available full-size mechanical keyboards with clicky switches:
\begin{itemize}
    \item Item ID \texttt{7706410293}: backlight ``none'', \$269.16
    \item Item ID \texttt{6342039236}: backlight ``white'', \$244.91
\end{itemize}
Unfortunately, there are no full-size mechanical keyboards with clicky switches and RGB backlighting currently in stock. Given your preference, the \texttt{7706410293} (\textbf{clicky, non-backlit}) seems to be the closest match. \\[0.5em]
... \\[0.5em]
\textbf{[Tool Call]:} \texttt{exchange\_delivered\_order\_items(new\_item\_ids=['7706410293', ...])} $\checkmark$
\end{tcolorbox}




\begin{tcolorbox}[
  colback=gray!5,
  colframe=gray!70,
  title=\textbf{22K Budget (Failure)},
  fonttitle=\bfseries\small,
  breakable
]
\textbf{[User]:} (Same request as above) \\[0.5em]
... \\[0.5em]
\textbf{[Assistant]:} I found an available full-size mechanical keyboard with clicky switches and RGB backlight (Item ID \texttt{9025753381}). However, it is currently out of stock. Alternatively, there is a full-size mechanical keyboard with clicky switches and \textbf{white backlight} (Item ID \texttt{6342039236}) available. Since you preferred RGB backlight, I will try to find one with RGB first. \textbf{If not available, I will proceed with the white backlight option.} \\[0.5em]
... \\[0.5em]
\textbf{[Tool Call]:} \texttt{exchange\_delivered\_order\_items(new\_item\_ids=['6342039236', ...])} $\times$
\end{tcolorbox}

\textbf{Analysis:} The user explicitly stated ``RGB or non-backlit''---white backlight was never an acceptable option. At 12K, the agent correctly interprets this constraint and selects the non-backlit keyboard. At 22K, despite having identical information, the agent invents a fallback logic (``if RGB unavailable, use white'') that contradicts the user's stated preference. The extended context allows the agent to ``overthink'' and rationalize an incorrect choice.

%==============================================================================
\paragraph{Case B: Input Over-Correction}
\begin{itemize}
    \item \textbf{Setting:} $\tau^2$-Bench, Retail Domain, Task 6, Gemini-2.5-Flash. User provides their name for account lookup.
\end{itemize}
Refer to Box~\ref{box:caseB-12k} and Box~\ref{box:caseB-22k}.

\begin{tcolorbox}[
  colback=gray!5,
  colframe=gray!70,
  title=\textbf{12K Budget (Success)},
  fonttitle=\bfseries\small,
  breakable
]
\textbf{[User]:} My name is Mei \textbf{Kovacs} and my zip code is 28236. \\[0.5em]
\textbf{[Tool Call]:} \texttt{find\_user\_id\_by\_name\_zip(first\_name="Mei", last\_name="Kovacs", zip="28236")} \\[0.5em]
\textbf{[Tool Result]:} \texttt{mei\_kovacs\_8020} $\checkmark$
\end{tcolorbox}


\begin{tcolorbox}[
  colback=gray!5,
  colframe=gray!70,
  title=\textbf{22K Budget (Failure)},
  fonttitle=\bfseries\small,
  breakable
]
\textbf{[User]:} My name is Mei \textbf{Kovacs} and my zip code is 28236. \\[0.5em]
\textbf{[Tool Call]:} \texttt{find\_user\_id\_by\_name\_zip(first\_name="Mei", last\_name="Kov\'{a}cs", zip="28236")} \\[0.5em]
\textbf{[Tool Result]:} \texttt{Error: User not found} $\times$
\end{tcolorbox}

\textbf{Analysis:} The user typed ``Kovacs'' (ASCII), but the 22K agent ``helpfully'' transformed it to ``Kov\'{a}cs'' with a Hungarian diacritic. This over-correction breaks the exact-match database lookup. With more context budget, the model applies world knowledge (Hungarian naming conventions) inappropriately, modifying user input that should have been passed verbatim.

%==============================================================================
\paragraph{Case C: Action Loops}
\begin{itemize}
    \item \textbf{Setting:} $\tau^2$-Bench, Telecom Domain, Mobile Data Troubleshooting Task, Gemini-2.5-Flash. User reports no mobile data while traveling abroad.
\end{itemize}
Refer to Box~\ref{box:caseC-12k} and Box~\ref{box:caseC-22k}.

\begin{tcolorbox}[
  colback=gray!5,
  colframe=gray!70,
  title=\textbf{12K Budget (Success) --- 29 tool calls},
  fonttitle=\bfseries\small,
  breakable
]

\texttt{1. get\_customer\_by\_phone} \\
\texttt{2-4. get\_details\_by\_id} (3$\times$) \\
\texttt{5. enable\_roaming} \\
\texttt{6. reboot\_device} \\
\texttt{7. disconnect\_vpn} \\
\texttt{8. set\_network\_mode\_preference} \\
\texttt{9. transfer\_to\_human\_agents} $\leftarrow$ \textit{called once, then continues} \\
\texttt{10. check\_data\_restriction\_status} \\
\texttt{11. disconnect\_vpn} \\
... \\
\texttt{29. run\_speed\_test} $\checkmark$ \textit{Problem resolved}
\end{tcolorbox}

\begin{tcolorbox}[
  colback=gray!5,
  colframe=gray!70,
  title=\textbf{22K Budget (Failure) --- 117 tool calls},
  fonttitle=\bfseries\small,
  breakable
]
\texttt{1. get\_customer\_by\_phone} \\
\texttt{2-4. get\_details\_by\_id, enable\_roaming, get\_data\_usage} \\
... \\
\texttt{18. transfer\_to\_human\_agents} \\
\texttt{19. transfer\_to\_human\_agents} \\
\texttt{20. reset\_apn\_settings, reboot\_device} \\
\texttt{22-23. run\_speed\_test} (2$\times$) \\
\texttt{24-117. transfer\_to\_human\_agents} (94$\times$) $\times$ \textit{Stuck in loop}
\end{tcolorbox}

\textbf{Analysis:} At 12K, the agent calls \texttt{transfer\_to\_human\_agents} once (step 9), receives a response indicating the transfer failed, and \emph{continues troubleshooting} with alternative approaches---eventually solving the problem. At 22K, the agent enters a loop of 96 consecutive \texttt{transfer\_to\_human\_agents} calls, never breaking out to try other solutions. The larger context budget provides more ``room'' for repetitive behavior, allowing the agent to persist in unproductive patterns rather than being forced to try alternatives.

%==============================================================================
\paragraph{Case D: Redundant Search Loops}
\begin{itemize}
    \item \textbf{Setting:} MCP-Bench, API Documentation Analysis Task, Gemini-2.5-Flash. User requests a security health check on two external API services, requiring validation against OAuth2 best practices from academic papers and community guides.
\end{itemize}
Refer to Box~\ref{box:caseD-64k} and Box~\ref{box:caseD-128k}.

\begin{tcolorbox}[
  colback=gray!5,
  colframe=gray!70,
  title=\textbf{64K Budget --- 33 rounds 105 tool calls},
  fonttitle=\bfseries\small,
  breakable
]

\textbf{[Task]:} Health check on OpenAI and GitHub API documentation. Validate schemas, check authentication mechanisms, compare against OAuth2 recommendations. \\[0.5em]
\textbf{Wikipedia Searches for ``OWASP'':} \\
\texttt{R3:} \texttt{search\_wikipedia("OWASP OAuth 2.0 Security Cheatsheet")} \\
\texttt{R7:} \texttt{search\_wikipedia("OWASP API Security Project")} \\
\texttt{R11-13:} \texttt{search\_wikipedia("OWASP API Security Top 10")} \\
\textit{Total: 10 OWASP-related searches across 33 rounds} \\[0.5em]
\textbf{ArXiv Searches for OAuth:} 21 queries, progressing from general to specific RFCs \\[0.5em]
\textbf{Execution:} 994 seconds, 1.78M tokens $\checkmark$
\end{tcolorbox}

\begin{tcolorbox}[
  colback=gray!5,
  colframe=gray!70,
  title=\textbf{128K Budget --- 127 rounds 329 tool calls},
  fonttitle=\bfseries\small,
  breakable
]
\textbf{[Task]:} Same as above \\[0.5em]
\textbf{Wikipedia Searches for ``OWASP'':} \\
\texttt{R6:} \texttt{search\_wikipedia("OWASP API Security Top 10 OAuth 2.0")} \\
\texttt{R10:} \texttt{search\_wikipedia("OWASP API Security Top 10")} \\
\texttt{R14:} \texttt{search\_wikipedia("OWASP API Security Top 10")} \\
\texttt{R17:} \texttt{search\_wikipedia("OWASP API Security Top 10")} \\
\texttt{R33:} \texttt{search\_wikipedia("OWASP API Security Top 10 summary")} \\
\texttt{R52:} \texttt{search\_wikipedia("OWASP API Security Top 10")} \\
\texttt{R63:} \texttt{search\_wikipedia("OWASP API Security Top 10")} \\
... \\
\textit{Total: 18 OWASP-related searches across 127 rounds} \\[0.5em]
\textbf{ArXiv Searches for OAuth:} \\
\texttt{R1:} \texttt{search\_arxiv("OAuth2 security recommendations recent")} \\
\texttt{R3:} \texttt{search\_arxiv("OAuth2 security vulnerabilities best practices")} \\
\texttt{R6:} \texttt{search\_arxiv("OAuth 2.0 security attacks vulnerabilities...")} \\
\texttt{R10:} \texttt{search\_arxiv("OAuth 2.0 security best practices")} \\
\textit{(same concept searched 6$\times$ with minor variations)} \\[0.5em]
\textbf{Execution:} 3,878 seconds (3.9$\times$ slower), 11.6M tokens (6.5$\times$ more) $\times$
\end{tcolorbox}

\textbf{Analysis:} The 128K agent exhibits \emph{exploration without consolidation}. With a larger context window, the agent can hold more retrieved information, but paradoxically this leads to \emph{more} searching rather than synthesis. The query ``OWASP API Security Top 10'' is searched 9 times across different rounds---each time the agent seems to ``forget'' it already has this information. The ArXiv search pattern shows the same concept (``OAuth 2.0 security best practices'') being queried with trivial variations 6 times. This redundant exploration consumes 6.5$\times$ more tokens while producing equivalent results, demonstrating that larger context budgets can enable inefficient ``wandering'' behavior that smaller budgets would prevent.
