# Supplementary material for: Evaluating Test-Time Scaling of General LLM Agents
Source: arXiv:2602.18998 source file (2026-09-29)
Supplement: Supplementary file 6 [file appendix_long_context.tex]

\begin{figure*}[t]
\centering
\includegraphics[width=1.0\linewidth]{figs/tau2_heatmap.png}
\caption{$\tau^2$-Bench score heatmap in sequential scaling.}
\label{fig:tau2-heatmap}
\end{figure*}
